# Supplementary material for: $k$-local Graphs
Source: arXiv:2410.00601 source file (2025-05-08)
Supplement: Supplementary file 1 [file appendixproofs.tex]

\ifpaper
\input{./proofs/npmembership}
\fi

\setcounter{theorem}{5}
\ifpaper
\begin{proposition}
	For an undirected graph $G$, the problem $\Loc_G$ is $\NP$-complete.
\end{proposition}
\input{./proofs/npcompleteness}
\fi

\ifpaper
\begin{theorem}
	For every undirected graph $G$, we have $\Loc_{G,1}\in\mathsf{P}$.
\end{theorem}
\input{./proofs/1locinP}
\fi

\ifpaper
\begin{proposition}
	For every graph $G=(V,E)$ there is a (valid) colouring~$c$ such that $\loc(G,c)=\gamma(G)$.
\end{proposition}
\input{./proofs/locequalnrconncomp}
\fi

\setcounter{theorem}{9}
\ifpaper
\begin{proposition}
	For every graph $G$ with colouring $c$ there exists a validly coloured (by $c$) induced minor $G'$ of $G$ such that	$\loc(G,c)=\loc(G',c)$.
\end{proposition}
\input{./proofs/onlycolouredgraphs}
\fi

\ifpaper
\begin{theorem}
	For all graphs $G$ coloured by $c$, we have $\gamma(G)\leq \loc(G,c)\leq \alpha(G)$.
\end{theorem}
\input{./proofs/independentset}
\else    % ONLY ARCHIVE
\fi

\setcounter{theorem}{12}
\ifpaper
\begin{proposition}
	Complete, star, wheel and friendship graphs are $1$-local independent of the colouring.
\end{proposition}
\input{./proofs/many1localgraphs}
\fi

\ifpaper
\begin{proposition}
	If $\ell \in \N_{\geq 2}$ is even, web graphs are $\frac{\ell r}{2}$-local for every valid $2$-colouring. If $\ell$ is odd, there exists a $3$-colouring such that $W_{\ell,r}$ is $(\ell \operatorname{div} 3) r$-local.
\end{proposition}
\input{./proofs/webgraphs}
\fi

\ifpaper
\begin{proposition}
	For a minimal valid colouring, sunflower graphs $S_d$ and helm graphs $H_d$ for $d\in \N$ are $\lfloor \frac{d-1}{2}\rfloor$-local.
\end{proposition}
\input{./proofs/sunflowergraphs}
\fi

\subsection{Bipartite Graphs}

\ifpaper
\begin{proposition}
	Let $G=(V_1\dot{\cup} V_2,E)$ be a $K_3$-free, i.e., bipartite, graph that is $2$-coloured. Then $G$ is strictly $\min\{|V_1|,|V_2|\}$-local.
\end{proposition}
\input{./proofs/bipartite1}
\fi

\ifpaper
\begin{corollary}
	For $d\in\N$, hypercubes $Q_d$ are strictly $2^{d-1}$-local, every knight's graph on $KG = (V_1\dot{\cup}V_2,E)$ and gear graphs $G_d$ are strictly $\min\{|V_1|,|V_2|\}$-local and $d$-crown graphs $(\{x_1, \cdots, x_d, y_1, \ldots, y_d\},\{(x_i,y_j) \mid i,j \in [d], i\neq j\})$ are strictly $d$-local for $d \in \N_{\geq 3}$.
\end{corollary}
\input{./proofs/bipartite2}
\fi

\setcounter{theorem}{19}
\ifpaper
\begin{proposition}
	Let $G=(V_1\dot{\cup} V_2,E)$ be a bipartite graph that is $(>2)$-coloured by a colouring $c$. If there exists a colour $x\in \mathcal{C}(G,c)$ such that for all $v \in V_i$ we have $c(v) = x$ for exactly one $i \in [2]$ and $|V_i| \leq |V_j|$ for $j \in [2] \setminus \{i\}$ then $G$ is strictly $|V_i|$-local. Otherwise $G$ is strictly $|V_j|$-local.
\end{proposition}
\input{./proofs/bipartite2}
\fi

\ifpaper
\begin{proposition}
	Let $\tilde{\Sigma} = \{\widetilde{\ta}_i \mid \ta_i \in \Sigma\}$. For all condensed $w \in \Sigma^*$ there exists $\tilde{w} \in (\Sigma \cup \tilde{\Sigma})^*$ such that for all $x \in \letters(w)$ we have either $\{i \mid w[i] = x\} \subset 2\mathbb{N}$ or $\{i \mid w[i] = x\} \subset 2\mathbb{N}+1$. Further, $w$ is strictly $k$-local iff $\tilde{w}$ is strictly $k$-local.
\end{proposition}
\input{./proofs/tildew}
\fi

\ifpaper
\begin{theorem}
	Let $G$ be a bipartite graph that is coloured by $c$ with more than $\ell>2$ colours. Then $(G,c,k)\in\Loc_G$ is $\NP$-complete.
\end{theorem}
\input{./proofs/bipartitenp}
\fi

\subsection{Snarks}
%\ifpaper
%\input{flowersnarks}
%\fi 
\setcounter{theorem}{24}
\ifpaper
\begin{proposition}
	For every flower snark $J_d$, $d\in 2\N +1$ there exists a $\chi(J_d)$-colouring such that $J_d$ is $(d - (d \operatorname{mod} 3))$-local.
\end{proposition}
\input{./proofs/flowersnarkproof}
\fi

We finish this section with an overview of the graph classes.

\begin{table}
	\centering
	\begin{tabular}{l|c|c}
		Class & Lower Bound & Upper Bound \\
		\hline
		\hline
		Complete Graphs, Star Graphs& $1$ & $1$\\
		Wheel Graphs, Friendship Graphs & &  \\
%		Wheel Graphs & & \\
%		 & & \\
		\hline
		Paths & $1$ & $\lfloor n/2 \rfloor$ \\
		Cycles, Web graphs &  & \\
		1/2-regular Graphs & & \\
		%		2-regular Graphs & & \\
%		Web graphs & & \\
		\hline
		Complete Bipartite Graphs $K_{n_1,n_2}$ & $1$ & $\min\{n_1,n_2\}$\\
		Crown Graphs, Hypercubes & & \\
		Bipartite Graphs with $2$-colouring & & \\
%		 & & \\
		Knight's graph, Gear graph & & \\
%		 & & \\
		\hline
		Sunflower graphs $S_d$, Helm graphs $H_d$ & 1 & $\lfloor \frac{d-1}{2} \rfloor$ \\
		\hline
		Peterson Graph & 1 & 3 \\
		\hline
		Edgeless Graphs, 0-regular Graphs & $n$ & $n$\\
%		 & & \\
	\end{tabular}
	\caption{A summary of upper and lower bounds for the locality of graph classes.}
	\label{tablegraphs}
\end{table}

\subsection{Naive Search}

We compared our proposed priority search algorithm (Algorithm \ref{alg:priority_search}) in section \ref{pract} as an improvement over the naive search, which enumerates all possible valid colour permutations and checks their respective $k$-locality.
It is defined as follows:

\begin{algorithm}[!h]
\caption{Naive Search}
\label{alg:na\"ivve_search}
    \Input{Graph $G = (V, E)$, colouring $c : V \to [\ell]$}
    \Output{minimum $k$-locality of $G$ and all marking sequences of that $k$locality}
    \nonl\hrulefill
    
    min$_k \gets \infty$ \;
    minSequences $\gets \emptyset$ \;
    \ForAll{valid colour permutations $\pi$ over $\mathcal C (G,c)$}{
        current$_k$, currentSequences $\gets$ $k$-locality$(G, p)$ \;
        \If{current$_k$ == min$_k$}{
            minSequences $\gets$ minSequences $\cup$ currentSequences \;
        }
        \If{current$_k$ < min$_k$}{
            min$_k \gets$ current$_k$ \;
            minSequences $\gets$ currentSequences \;
        }
    }
    \Return min$_k$, minSequences \;
\end{algorithm}

\subsection{Priority Search}

In order to prove Theorem \ref{priority_search_optimality}, we must first show three additional properties.
We also use the following notation:
Let $\kappa$ denote the minimum $k$-locality of $G$ for any marking sequence.
Let $M$ be the set of all marking sequences $e$ with $\loc(G,e) = \kappa$.
Let $M'$ be the set of all marking \textit{prefixes} that can be expanded directly (i.e., by adding a single colour) to a marking sequence in $M$.

\setcounter{theorem}{54}
\ifpaper 
\begin{lemma}\label{priority_search_lemma1}
    Every correct $k$-locality algorithm must at least expand all marking prefixes that have a $k$-locality of $\kappa$.
\end{lemma}

\begin{proof}
    Assume that a marking prefix $p$ with $\loc(G,p) \leq \kappa$ is not expanded by a correct algorithm.
    Then it is still possible for an expansion $p'$ of $p$ to have $\loc(G, p') \leq \kappa$.
    The minimum $k$-locality of $G$ w.r.t. all marking sequences could not be validated, and $p'$ (or an expansion thereof) could be part of the result (i.e., $M$).
    This would violate the assumption of correctness.
\end{proof}

\begin{lemma}\label{priority_search_lemma2}
    All marking prefixes are expanded in ascending order of their $k$-locality.
\end{lemma}

\begin{proof}
    All marking prefixes are expanded in the order they are taken from the queue.
    Since the queue is always maintained sorted in ascending order w.r.t.~the $k$-locality, they are taken from the queue in ascending order.
    As a result, we must ensure that no marking prefix $p'$ with lower $k$-locality than a previously accessed marking prefix $p$ is added into the queue (where it later could be accessed and expanded again, violating the expansion in ascending order).
    If a marking prefix $p''$ was taken from the queue after $p$, it was either sorted behind $p$ because it had a greater or equal $k$-locality to begin with, or it is an expansion of $p$, in which case it cannot have lower $k$-locality, since current$_k$ in line 9 can never shrink.
    Therefore, all marking prefixes that are added to the queue later must have a greater or equal $k$-locality, ensuring that the marking prefixes are accessed and expanded in ascending order w.r.t.~the $k$-locality.
\end{proof}

\begin{lemma}\label{priority_search_lemma3}
    No marking prefix $p$ is expanded with $\loc(G,p) > \kappa$.
\end{lemma}

\begin{proof}
    The variable min$_k$ is only set once a marking prefix is expanded to a complete marking sequence $e$.
    If $\loc(G, e) = \kappa$, the condition in line 4 guarantees that no further marking prefixes with larger $k$-locality are expanded.
    If $\loc(G,e) > \kappa$, then, according to Lemma \ref{priority_search_lemma2}, the $k$-locality of its un-expanded version must have had a lower $k$-locality than any marking prefix in $M'$, since it was expanded first.
    As such, the prefix of $e$ must have had a $k$-locality of at most $\kappa$.
\end{proof}

\setcounter{theorem}{27}
\begin{theorem}
    Algorithm \ref{alg:priority_search} is optimal in the number of successive expansions of a marking prefix beginning with an empty sequence.
\end{theorem}

\begin{proof}
    According to Lemma \ref{priority_search_lemma1} we must continue to expand marking prefixes, as long as incomplete marking prefixes remain at the front of the queue with $k$-locality less than $\kappa$.
    According to Lemma \ref{priority_search_lemma2} the relevant marking prefixes reside at the front of the queue and are expanded from there.
    According to Lemma \ref{priority_search_lemma3}, the marking prefixes are expanded as long as they have a $k$-locality less than or equal to $\kappa$.
    In total, this proves that Algorithm \ref{alg:priority_search} guarantees correct results, since it expands at least all necessary marking prefixes, and is optimal, because it never expands any unnecessary marking prefixes.
\end{proof}

\begin{remark}
    It is worth noting that the priority*-variant of Algorithm \ref{alg:priority_search} does not quite satisfy the condition for the proof of Lemma \ref{priority_search_lemma1}, since not all marking prefixes are expanded to find all marking sequences in $M$.
    However, the guarantees of correctness and optimality for the minimal $k$-locality $\kappa$ still hold.
\end{remark}

\fi
